# Supplementary material for: Algorithmic approach to diagrammatic expansions for real-frequency evaluation of susceptibility functions
Source: arXiv:2004.11091 ancillary file (2020-04-23)
Supplement: Supplementary file 1 [file Supplemental_Materials__Susceptibility.pdf]

# Supplemental Materials: Algorithmic approach to diagrammatic expansions for real-frequency evaluation of susceptibility functions

Amir Taheridehkordi,[1] S. H. Curnoe,[1] and J. P. F. LeBlanc[1,*]

[1]*Department of Physics and Physical Oceanography, Memorial University of Newfoundland, St. John's, Newfoundland & Labrador, Canada A1B 3X7*

(Dated: April 22, 2020)

## RESULTS ON THE MATSUBARA FREQUENCY AXIS

### A higher temperature example

In Fig. S1 we plot the transverse spin susceptibility versus Matsubara frequency at a relatively high temperature $\beta t = 2.5$ and a weak coupling $U/t = 2$ (Fig. 2 in the main text uses $\beta t = 5$). The direct third order approximation is in solid agreement with the results from self-consistent ladder dual-fermion (DF) calculations.

### Temperature dependence for a non-zero Matsubara frequency

As illustrated in Fig. 3 in the main text, upon decreasing temperature, a higher order truncated series should be considered to obtain numerically reliable results. However, one should note that convergence away from zero frequency is quite fast and the third order approximation is typically sufficient. To demonstrate this we present the transverse susceptibility at the first Matsubara frequency against inverse temperature order at $U/t = 1$ and $U/t = 2$ for $m_c = 0$ to 3. We find that, at these interaction strengths, even at the extremely low temperature $\beta t = 11$ the second and third order approximation are almost identical, i.e., the third order approximation is sufficient to approximate the susceptibility function. Moreover, in both cases the agreement with DF is solid.

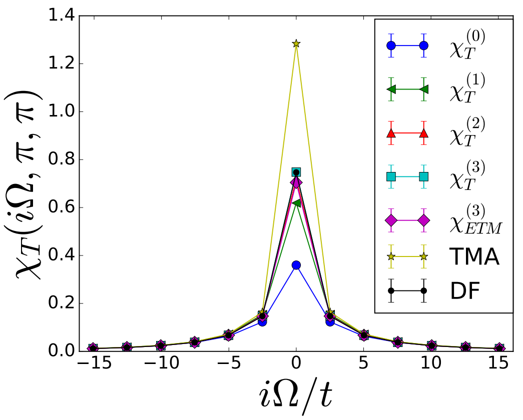


Figure S1. Transverse spin susceptibility vs. Matsubara frequency $i\Omega$ at different truncation orders $m_c = 0$ to 3. Data are for $U/t = 2$, $\beta t = 2.5$ with $\mu/t = 0$ at $\mathbf{q} = (\pi, \pi)$. We show the third order ETM, TMA and DF results for comparison.

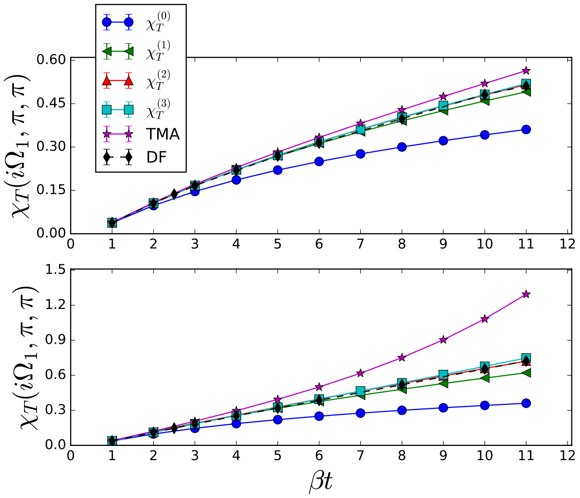


Figure S2. Transverse spin susceptibility vs. inverse temperature at different truncation orders $m_c = 0$ to 3. The TMA and DF results are also shown for comparison. Data are for *Top*: $U/t = 1$, *Bottom*: $U/t = 2$ with $\mu/t = 0$ at $\mathbf{q} = (\pi, \pi)$ and $i\Omega = i\Omega_1 = 2\pi/\beta$.

## RESULTS ON THE REAL FREQUENCY AXIS

### Order-by-order contribution

In Fig. S3 we show the order-by-order contribution of diagrams $[O(m)]$ with $m = 0$ to 3 to the transverse spin susceptibility versus real frequency for $\beta t = 5$, $U/t = 1$, and $\mu/t = 0$ at $\mathbf{q} = (\pi/3, \pi/2)$. We find that high order terms mostly contribute for a range of frequencies near $\Omega = 0$ and also near the band edge above $\omega = 4$. Furthermore, as one expects the higher order contributions decay very fast increasing order (Fig. 4 of the main text shows the imaginary part only, for a larger value of $U/t = 2$).

We also show in Fig. S4 the order-by-order contribution to real part of the susceptibility function at $U/t = 2$ with the same parameters as the main text Fig. 4. One immediately notes that in this parameter regime, the con-

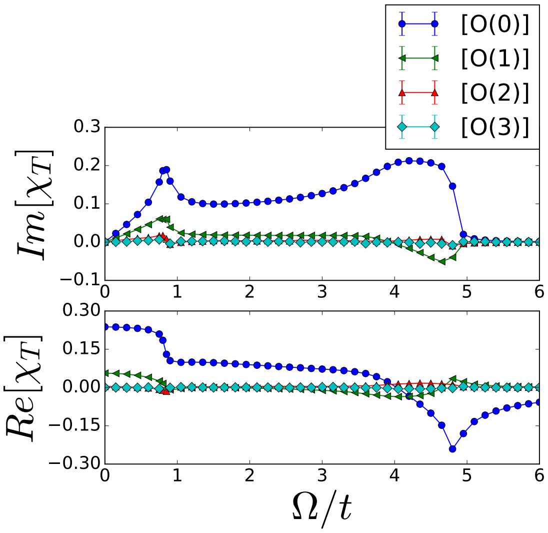


Figure S3. *Top*: imaginary and *Bottom*: real part of the $m$th order transverse spin susceptibility diagrams $[O(m)]$ vs. real frequency $\Omega$. Data are for $\beta t = 5$, $U/t = 1$, and $\mu/t = 0$ at $\mathbf{q} = (\pi/3, \pi/2)$. We set $\Gamma/t = 0.02$ in the symbolic analytic continuation $i\Omega \to \Omega + i\Gamma$.

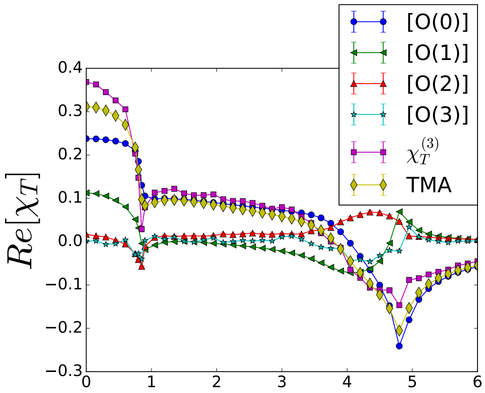


Figure S4. Real part of the $m$th order transverse spin susceptibility diagrams vs. real frequency $\Omega$. The TMA and third order transverse spin susceptibility $\chi_T^{(3)}$ are also shown. Data are for $\beta t = 5$, $U/t = 2$, and $\mu/t = 0$ at $\mathbf{q} = (\pi/3, \pi/2)$. We set $\Gamma/t = 0.02$ in the symbolic analytic continuation $i\Omega \to \Omega + i\Gamma$.

tribution of the second and third order diagrams is negligible for $1.5 < \Omega < 3$ and $\Omega > 5$.

## Comparison with TMA

In Fig. S5 we compare the second order transverse spin susceptibility, $\chi_T^{(2)}$ with TMA on the real frequency axis for different choices of $U/t = 1 \to 3$. We note that by increasing $U/t$ the peak in $\mathrm{Im}[\chi_{TMA}]$ moves to lower $\Omega$ and the peak becomes rounded, a behavior not observed in $\chi_T^{(2)}$ where the peak is independent of the choice of $U/t$ and remains sharp. Moreover, TMA results show a much steeper slope in vicinity of $\Omega = 0$ compared to the second order approximation.

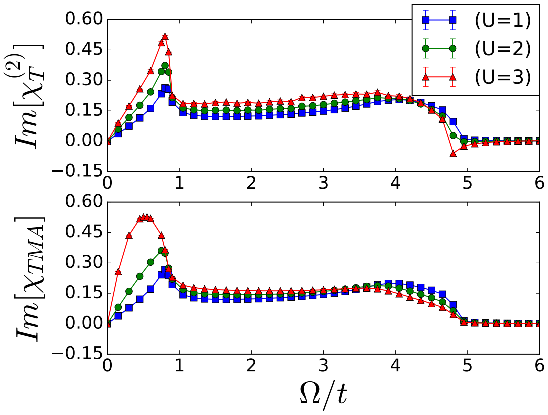


Figure S5. Imaginary part of the second order and TMA transverse spin susceptibility vs. real frequency $\Omega$ for $U = 1 \to 3$. Data are for $\beta t = 5$ and $\mu/t = 0$ at $\mathbf{q} = (\pi/3, \pi/2)$. We set $\Gamma/t = 0.02$ in the symbolic analytic continuation $i\Omega \to \Omega + i\Gamma$.

## Analytic continuation: dependence on the regulator

We investigate the dependence of the first order transverse susceptibility function on the regulator $\Gamma$ in Fig. S6 for $\beta t = 5$, $U/t = 2$, and $\mu/t = 0$ at $\mathbf{q} = (\pi/3, \pi/2)$ and $\Omega/t = 2$. We observe that the result has only weak dependence on $\Gamma/t \leq 0.04$. Therefore, our choice of regulator in this work $\Gamma/t = 0.02$ is effectively in the limit of $\Gamma \to 0$.

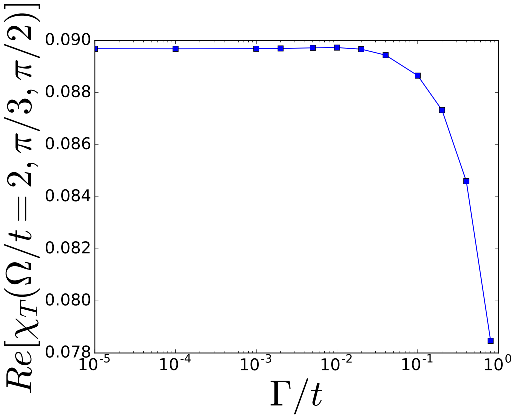


Figure S6. Real part of the first order transverse spin susceptibility vs. regulator $\Gamma$ in analytic continuation process $i\Omega \to \Omega + i\Gamma$. Data are for $\beta t = 5$, $U/t = 2$, and $\mu/t = 0$ at $\mathbf{q} = (\pi/3, \pi/2)$ and $\Omega/t = 2$.

* jleblanc@mun.ca
